# Supplementary material for: BlindMarket: Enabling Verifiable, Confidential, and Traceable IP Core Distribution in Zero-Trust Settings
Source: arXiv:2603.22685 source file (2026-03-24)
Supplement: Supplementary file 1 [file appendix.tex]

\newpage 
\appendix
\section{Appendix}
\subsection{Soft IP Metadata Records}\label{ap:metadata}
See Table~\ref{tab:softip-attributes}

\subsection{License Authorization}\label{ap:license}
% \subsubsection{Formalized Public-key Signature.}
% A public-key signature scheme provides authenticity, integrity, and non-repudiation for digital messages through three core algorithms:  
% \begin{itemize}[label={$-$},leftmargin=15pt]
%     \item {\sf KeyGen}(\(1^\lambda\)) \(\rightarrow\) (\(\mathsf{sk}, \mathsf{pk}\)): Generates a secret signing key \(\mathsf{sk}\) and a public verification key \(\mathsf{pk}\) based on security parameter \(\lambda\).
    
%     \item \textsf{Sign}(\(\mathsf{sk}, m\)) \(\rightarrow\) \(\sigma\): Outputs a signature \(\sigma\) for message \(m\) using \(\mathsf{sk}\).
    
%     \item \textsf{Verify}(\(\mathsf{pk}, m, \sigma\)) \(\rightarrow\) \{0,1\}: Outputs 1 if \(\sigma\) is a valid signature for \(m\) under \(\mathsf{pk}\), else 0.
% \end{itemize} 

\subsubsection{Record generation for IP usage authentication.}
\label{sec:ip-auth}
\begin{flalign*}
&\mathcal{R} \gets \bigl( ID, \mathcal{H}(D),\, addr_v,\, addr_u,\, \{\} \bigr) \\
&(sk_v, pk_v) \gets \textsf{KeyGen}(1^u) \quad
\sigma_v \gets \textsf{Sign}(sk_v,\mathcal{R})) \quad
\textsf{PushRecord}\bigl( \mathcal{R}, \sigma_v \bigr)
\end{flalign*}

\subsubsection{Record generation for IP registration.}
\label{sec:ip-regist}
\begin{align*}
&\mathcal{R} \gets \bigl(ID, \mathcal{H}(D),\, addr_u,\, addr_u,\, \{ID_i,\, ID_j\}\bigr) \\
&(sk_u, pk_u) \gets \textsf{KeyGen}(1^u) \quad
\sigma_u \gets \textsf{Sign}(sk_u,\mathcal{R})) \quad
\textsf{PushRecord}\bigl( \mathcal{R}, \sigma_u \bigr)
\end{align*}

\subsubsection{Authenticated IP usage trace.}

See Algorithm~\ref{alg:trackIP}
\label{sec:ip-trace}
\begin{algorithm}[h]
\caption{traceSoftIP}
\label{alg:trackIP}
\begin{algorithmic}[1]
\Require A design identifier \( ID \)
\Ensure The orignial Vendors \(\set{D}\)
    \State \(R \gets \textsf{TrackRecord}(ID)\)
    \State $ pk \gets \textsc{retrievePubKey}(R.\text{From})$
    \State $ \textbf{Assert} (\textsc{Verify}(pk,R.\text{SoftIPMetaData},R.\sigma) )$
    \If{\(R.\texttt{Reference} = \varnothing\)}
        \State \Return \(\{R.\texttt{From}\}\)
    \Else
        \State \(\set{D} \gets \varnothing\)
        \ForAll{\(ID' \in R.\texttt{Reference}\)}
            \State $\set{D} \gets \set{D} \cup \Call{traceSoftIP}{ID'}$
        \EndFor
    \EndIf
\end{algorithmic}
\end{algorithm}

\subsection{Secure Design Verification}\label{ap:secureIPverif}
See Algorithm~\ref{alg:designverif}
\begin{algorithm}[h]
\caption{2PC-Based Design Verification}
\label{alg:designverif}
\begin{algorithmic}[1]
\Require User: $(\randomize{P}_i, \randomize{N}_i),\ \varphi$; \quad Vendor: $(R_P, R_N)$
\Ensure $\texttt{result} \in \{\texttt{SAT}, \texttt{UNSAT}\}$

\State User computes $(\varphi_P, \varphi_N) \gets \textsc{Encode}(\neg \varphi)$
\State Jointly reconstruct encoded design: 
\[
(\secret{P_i}, \secret{N_i}) \gets (\secret{\randomize{P}_i} \oplus \secret{R_P},\ \secret{\randomize{N}_i} \oplus \secret{R_N})
\]
\State Construct verification instance:
\[
(\secret{P'}, \secret{N'}) \gets (\secret{P_i}~\|~\secret{\varphi_P},\ \secret{N_i}~\|~\secret{\varphi_N})
\]
\State $\texttt{result} \gets \texttt{ppSAT.Solve}(\secret{P'}, \secret{N'})$
\end{algorithmic}
\end{algorithm}
\begin{figure}[b]
    \centering
\includegraphics[width=.5\linewidth]{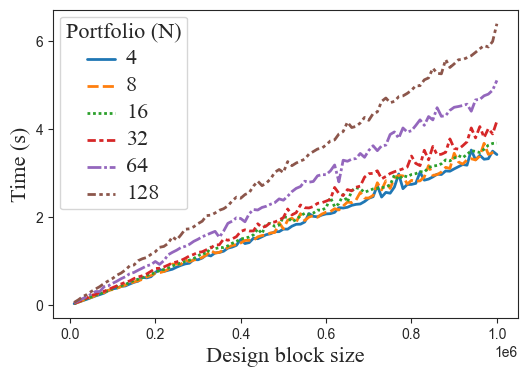}
    \caption{1 out of N OT scales linearly with the formula size.}
    %\vspace{-0.15in}
    \label{fig:ot_formula}
\end{figure}

\subsection{Evaluation of Oblivious IP Selection}\label{ap:evalot}
See Figure~\ref{fig:ot_formula}

% \subsection{Related Work}\label{ap:related}

% Table~\ref{tab:quantitativecomp} lists the summary of the existing work and its limitations.

% \begin{table}[h]
%     \centering
%         \caption{Existing methods cannot provide privacy protection for formal-based IP verification without a third party.}
%     \begin{tabular}{cccc}
%     \toprule
%     \textbf{Approach} & \textbf{Parties} & \textbf{Verification} & \textbf{Stage}\\
%     \midrule
%     TIPP~\cite{kahng2001constraint,alkabani2007active,kamali2022advances} &- & - &\textit{Post-fabrication} \\
%     % \midrule
%     IEEE 1735~\cite{7274481} & 3& Simulation/Synthesis &\textit{Pre-silicon} \\
%     % \midrule
%     Garbled EDA~\cite{hashemi2022garbled} & 3 & Simulation& \textit{Netlist}\\
%     % \midrule
%     MP$\ell$$\circ$C~\cite{mouris2023mploc} &2 & Simulation & \textit{Netlist}\\
%     % \midrule
%         Pythia~\cite{mouris2020pythia} &2 & Simulation & \textit{Netlist}\\
%     \textbf{This Work} & \textbf{2} &\textbf{Formal Logic}  & \textbf{RT-Level}\\
%     \bottomrule
%     \end{tabular}

%  %\ning {this table should be moved forward, along with technique challenge and contribution.}\liu{move back as Section 2}
%     \label{tab:quantitativecomp}
% \end{table}
