# Supplementary material for: BlindMarket: Enabling Verifiable, Confidential, and Traceable IP Core Distribution in Zero-Trust Settings
Source: arXiv:2603.22685 source file (2026-03-24)
Supplement: Supplementary file 2 [file supplementary.tex]

\newpage
\makeatletter
\setcounter{section}{0}
\renewcommand\thesection{\@arabic\c@section}
\setcounter{subsection}{1}
\renewcommand\thesubsection{\thesection.\@arabic\c@subsection}
\makeatother
\input{sections/benchmark}

\begin{center}  
\section{Supplementary material}
\end{center}

\subsection{Revise on Cryptographic Tools}
We consider {ppSAT} as consisting of two phases: the {\bf sharing} (\texttt{ppSAT.share}) phase and the {\bf solving} (\texttt{ppSAT.solving}) phase.  Each party first encodes its private Boolean formula as a pair of matrices, denoted by \( (P_a, N_a) \) and \( (P_b, N_b) \), respectively. 
In the sharing phase, the two parties secret-share the concatenated matrices using Yao’s sharing~\cite{yao1986generate}. A value \( v \) is said to be \emph{Yao-shared}, denoted by \( \secret{v} \), if it is the output of a GC-based 2PC computation and has not been revealed to either party. In other words, the value still remains secret throughout the protocol execution. 
In the subsequent solving phase, \texttt{ppSAT} performs SAT solving by updating the shared matrix representation within 2PC framework.  Each update is referred to as a \emph{giant step}, which consists of three procedures: \emph{unit propagation}, \emph{pure literal elimination}, and \emph{variable decision branching}. In particular, \emph{variable decision branching} relies on an external heuristic to determine which variable assignment to try when no variable can be directly decided, and the solving process must proceed by branching.

\begin{figure}[h]
\label{app:matrix}
\centering
    \begin{align*}
P &= ~\begin{bNiceArray}{ccc}[first-row,last-col]
 C_1 & C_2 & C_3 &  \\
  1& 0 & 0 & ~x_1\\
  0&  0 & 1 & ~x_2\\
 0&  1 & 0 & ~x_3
\end{bNiceArray}
&
N &= ~\begin{bNiceArray}{ccc}[first-row,last-col]
 C_1 & C_2 & C_3 &  \\
 0&1 & 0 & \neg x_1 \\
1&  0 & 0 & \neg  x_2 \\
 0&  0 & 1 &\neg x_3 
\end{bNiceArray}
\end{align*}
\caption{Encoding of $\underbrace{(x_1 \lor \lnot x_2)}_{C_1} \land \underbrace{(\lnot x_1 \lor x_3)}_{C_2} \land \underbrace{(x_2 \lor \lnot x_3)}_{C_3}$.
}
\end{figure}
\subsection{Revise on Formulae Generation of Design.}
On the IP vendor side, the design is encoded as a Boolean formula through the following steps.  
Static analysis extracts a word-level intermediate representation of the design's behavior, which is then translated into a quantifier-free bit-vector SMT formula (QF-BV)~\cite{barrett2010smt}, where each variable is modeled as a \emph{fixed-size bit vector}.  
For instance, in Example~\ref{fig:rtlcounter}, the signal \signalname{counter}, defined starting at line~3, is translated into its corresponding SMT bit-vector representation beginning at line~10. 
The resulting SMT formula is then converted into conjunctive normal form (CNF) via \emph{bit-blasting} and \emph{Tseytin transformation}.  
Bit-blasting translates bit-vector operations into Boolean logic, while the Tseytin transformation encodes Boolean formulas in CNF using auxiliary variables without exponential growth. In contrast, existing hardware synthesis flows such as~\cite{wolf2016yosys}, which flatten the design into a netlist, require auxiliary signals to represent bit-vector operations. This, in turn, introduces significant overhead in \texttt{ppSAT}.

% Traditional synthesis flows flatten the design into primitive logic cells, requiring auxiliary signals to handle complex word-level operations. 
% \ning{add something} combinational statements as constraints over these vectors, and sequential statements modeled as assignments.\ning{add sequential statement example.} 
% These sequential statements are instantiated for a certain number of iterations to achieve soundness under bounded unrolling. \ning{rewrite grammar.}
% For bounded verification, the SMT formula is unrolled to a fixed bound by instantiating the transition relation over time.  

The vendor then constructs a semantic map for the \textit{observable signal}, as shown in lines~15–16, where each bit of the variables \signalname{counter} and \signalname{reset} is assigned a unique Boolean literal. This mapping enables the IP user to formulate properties in Section~\ref{subsec:ipspec}.
% including their bit-level identifiers, to enable the IP user to formulate the property in Section~\ref{subsec:ipspec}.
% Traditional synthesis flows flatten the design into primitive logic cells, requiring auxiliary signals to handle complex word-level operations.  
% In contrast, our direct SMT-based encoding avoids this overhead and generates a smaller Boolean formula.
% The workflow begins by obtaining a set of intermediate word-level representations of the statements of hardware design. A statement in hardware designs is either a sequential statement or a combinational statement.
% The sequential statement updates the hardware register by clock edge, which could be mapped to the next state function in SMT. 
% The combinational statement is mapped to a propositional logical constraint. 
% \ning{either talk about signals before or here. We should explain what sequential statements and combinational statements are in the preliminaries. We should also define control expression either in preliminaries or here.  }
The signals used in the control expressions are also tracked in the semantic map (such as \texttt{reset} in Example~\ref{fig:rtlcounter} line~2), which remains private. 
Each control signal is weighted by its depth in its statement's abstract syntax tree, and each bit of the control logic is leveraged to accelerate the SAT solver, as detailed in Section~\ref{sec:heuristics}.
{Example}~\ref{fig:rtlcounter} demonstrates how a simple counter with control signal \signalname{reset} and \signalname{enable} can be modeled using this methods symbolically.
The SMT constraints in lines 10–13 specify an equivalent logical formula that encodes its behavior. Specifically, the bit-vector \signalname{counter\#2} represents the symbolic variable of \signalname{counter} at the second clock cycle, while the expression is constructed using nested ternary operations. \signalname{counter\#1} refers to the symbolic variable of \signalname{counter} at the first clock cycle.
Furthermore, the vendor provides a semantic map that associates the 3-bit signal \signalname{counter\#2} with the literal $\{\ell_{4},\ell_{3},\ell_{2}\}$ and the 1-bit signal \signalname{reset\#1} with $\ell_1$, while also recording the depths of \signalname{reset\#1} and \signalname{enable\#1} as 1 and 2, respectively.

\begin{example}{Incrementing counter with synchronous reset}
\begin{lstlisting}[style=motivating,basicstyle=\ttfamily\scriptsize]
  always @(posedge clk) begin
    if (reset)
      counter <= 3'b0; // Reset the counter to 0
    else if (enable)
      counter <= counter + 3'b10; // Increment the counter by 2
    else
      counter <= counter + 3'b1; // Increment the counter by 1
  end
/* SMT Formulae */
counter#2 <--> (ite (= |reset#1| #b1)
#x00(ite (= |enable#1| #b1)
    (bvadd |counter#1| #x02)
    (bvadd |counter#1| #x01)))
/* semantic map */
{reset#1 : 1, counter#2[0] : 2, 
counter#2[1] : 3, counter#2[2] : 3} 
\end{lstlisting}
\label{fig:rtlcounter}
\end{example}
\subsection{Restatement of the verfied Property}
We restrict our specification fragment to three SVA temporal operators widely used in hardware verification: Overlap Implication (OI), Non-Overlap Implication (NOI), and Concatenation (Concat)~\cite{dobis2024formal}. 
These operators form the basis for temporal relationships within bounded execution traces. 
Specifically, OI (\(\mathrm{A} \svaNImpl \mathrm{B}\)) asserts that whenever A holds, B must hold at the same clock cycle, whereas NOI (\(\mathrm{A} \svaOImpl \mathrm{B}\)) requires B to hold in the next clock tick if A holds in the current clock tick. The Concat operator (\(\mathrm{A} \svaConcat{\mathrm{N}} \mathrm{B}\)) checks that A must be true on the current clock tick and B on the N$^{\text{th}}$ clock tick. Here, A and B are boolean expression defined as a sequence~\cite{vijayaraghavan2005practical}.

\subsection{Restatement of Experimental Metric}
Table~\ref{tab:exp} summarizes the performance evaluation of our control-flow-guided heuristics. For each (pruned) design pair, we report detailed measurements for each step of the protocol. The table columns are explained as follows:

\begin{itemize}[label={$-$},leftmargin=5pt]
    \item \texttt{Var/Cls}: Reports the size of the Boolean formula used in verification, expressed as the number of variables and clauses in the conjunction of the design and its specification.
    
    \item \texttt{OT Design Matrix}: Denotes the size of the design matrix that must be transferred via oblivious IP selection. Each block is 128b.
    
    \item \texttt{OT(1/32)(ms)}: Indicates the execution time for oblivious transfer, assuming a 1-out-of-32 OT protocol.
    
    \item \texttt{Deobfuscate(s)}: Records the time required to reconstruct the design metric using secure two-party computation (2PC), as defined in Equation~\ref{eq:deobfuscate}.
    \item \texttt{DLIS}: Reports the number of giant steps taken during SAT solving under the DLIS heuristic.    
    \item \texttt{ppsat(s)}: Measures the total SAT solving time using the standard DLIS heuristic.
     
    \item \texttt{Ctrl}: Records the number of giant steps taken under the control-guided heuristic.   
    
    \item \texttt{hw-ppsat(s)}: Represents the total solving time using our proposed control-flow-guided heuristic.
\end{itemize}

We highlight two types of performance improvements in this evaluation: (1) time reductions due to design pruning, and (2) improvements from heuristic guidance, reflected in the reduced number of giant steps (see Section~\ref{subsec:overviewppsat}). These optimizations collectively enhance the scalability and efficiency of our verification workflow.
\subsection{Extended Benchmark Setup.}
We provide more details about the experiment setup in
Table~\ref{tab:source}, which documents the benchmark suite: for each design, we report its source, Verilog lines of code (LOC), the SystemVerilog assertion (SVA), and a brief description.
